# Supplementary material for: Theory for the Charge-Density-Wave Mechanism of 3D Quantum Hall Effect
Source: arXiv:2003.02520 source file (2020-11-10)
Supplement: Supplementary file 1 [file CDW_supp_20200828.pdf]

# Supplemental Material

Fang Qin (覃昉),[1,2,3] Shuai Li,[1] Z. Z. Du,[1,4] C. M. Wang,[5,1,4]
Wenqing Zhang,[1,3] Dapeng Yu,[1,4] Hai-Zhou Lu,[1,4,*] and X. C. Xie[6,7,8]

[1] *Shenzhen Institute for Quantum Science and Engineering and Department of Physics, Southern University of Science and Technology (SUSTech), Shenzhen 518055, China*
[2] *CAS Key Laboratory of Quantum Information, University of Science and Technology of China, Chinese Academy of Sciences, Hefei, Anhui 230026, China*
[3] *Shenzhen Municipal Key-Lab for Advanced Quantum Materials and Devices, Shenzhen 518055, China*
[4] *Shenzhen Key Laboratory of Quantum Science and Engineering, Shenzhen 518055, China*
[5] *Department of Physics, Shanghai Normal University, Shanghai 200234, China*
[6] *International Center for Quantum Materials, School of Physics, Peking University, Beijing 100871, China*
[7] *CAS Center for Excellence in Topological Quantum Computation, University of Chinese Academy of Sciences, Beijing 100190, China*
[8] *Beijing Academy of Quantum Information Sciences, West Building 3, No. 10, Xibeiwang East Road, Haidian District, Beijing 100193, China*

(Dated: October 8, 2020)

In this Supplemental Material, we provide the detailed calculations for the results in the main text.

## CONTENTS

SI. Single-particle Hamiltonian S1

SII. Quantum limit S2

SIII. Linearization S3

SIV. Mean-field approach S4
A. Electron-electron interaction S4
B. Electron-phonon interaction S5

SV. Ground-state energy and period of the CDW state S6

SVI. Gap equation S8
A. Density of state for CDW S8
B. Zero-temperature case S8
C. Finite-temperature case S9

SVII. Lattice Ionic potential energy S10

SVIII. Tunneling current along the direction of magnetic field S10
A. Density of states S10
B. Non-Ohmic character along the $z$-direction S11

References S12

## SI. SINGLE-PARTICLE HAMILTONIAN

Motivated by the experiment [1], we will consider a low energy model of $ZrTe_5$ under a uniform magnetic field $\mathbf{B} = B\mathbf{e}_z$ along the $z$ direction (crystal $b$ direction), which can be described by a Landau gauge vector potential $\mathbf{A} = (-By, 0, 0)$.

* Corresponding author: luhz@sustech.edu.cn

In the basis $\hat{\Psi}^{\dagger}_{\mathbf{k}} = (\hat{a}^{\dagger}_{\mathbf{k},+,\uparrow}, \hat{a}^{\dagger}_{\mathbf{k},+,\downarrow}, \hat{a}^{\dagger}_{\mathbf{k},-,\uparrow}, \hat{a}^{\dagger}_{\mathbf{k},-,\downarrow})$ and Landau gauge $\mathbf{A} = (-By, 0, 0)$, the low-energy single-particle Hamiltonian density for $ZrTe_5$ is given by [2–4]

$$\hat{\mathcal{H}}(\mathbf{k}) = m\tau_z \otimes \sigma_0 + \hbar v_x \left(k_x - \frac{eB}{\hbar}y\right)\tau_x \otimes \sigma_z + \hbar v_y k_y \tau_y \otimes \sigma_0 + \hbar v_z k_z \tau_x \otimes \sigma_x, \tag{S1}$$

where, in a magnetic field along the $z$ direction, the wave vector $k_z$ is still a good quantum number, $k_{x/y}$ can be expressed as $k_{x/y} = -i\partial_{x/y}$, the Dirac mass is [3]

$$m = M_0 + M_1\left[v_x^2\left(k_x - \frac{eB}{\hbar}y\right)^2 + v_y^2 k_y^2\right] + M_z k_z^2 = M_0 + M_1\left[v_x^2\left(-i\partial_x - \frac{eB}{\hbar}y\right)^2 - v_y^2\partial_y^2\right] + M_z k_z^2, \tag{S2}$$

$M_0$, $M_1$, $M_z$, $v_{x,y,z}$ are the model parameters, $e$ is elementary charge, $B$ is the magnetic field, $\hbar$ is the reduced Planck's constant, $\hat{a}^{\dagger}_{\mathbf{k},j,\sigma}$ and $\hat{a}_{\mathbf{k},j,\sigma}$ are the creation and annihilation operators for the basis state $|\tau_z = \pm 1, S_z = \pm\frac{1}{2}\rangle$, $j = \pm$ are the pseudo orbital degrees, $\sigma = \uparrow, \downarrow$ is the pseudo spin symbol, $\tau_{x,y,z,0}$ and $\sigma_{x,y,z,0}$ are Pauli matrices and unit matrix operating on orbital and spin degrees of freedom.

Using the Landau gauge $\mathbf{A} = (-By, 0, 0)$ and the ladder operators with $v_x v_y B > 0$ [2, 3]

$$\hat{c} = \frac{\ell_B}{\sqrt{2}v_\perp}\left[v_x\left(k_x - \frac{eB}{\hbar}y\right) - iv_y k_y\right] = -\frac{\ell_B}{\sqrt{2}v_\perp}\left[v_x\left(i\partial_x + \frac{eB}{\hbar}y\right) + v_y\partial_y\right], \tag{S3}$$

$$\hat{c}^{\dagger} = \frac{\ell_B}{\sqrt{2}v_\perp}\left[v_x\left(k_x - \frac{eB}{\hbar}y\right) + iv_y k_y\right] = -\frac{\ell_B}{\sqrt{2}v_\perp}\left[v_x\left(i\partial_x + \frac{eB}{\hbar}y\right) - v_y\partial_y\right], \tag{S4}$$

where $v_\perp = \sqrt{v_x v_y}$ and $\ell_B = \sqrt{\hbar/(eB)}$ is the magnetic length.

Denote the normalized scalar eigenfunction of $\hat{c}^{\dagger}\hat{c}|n\rangle = n|n\rangle$ as $|n\rangle$. With the trial wave function $(|n-1\rangle, |n\rangle, |n\rangle, |n-1\rangle)^T$, $\hat{c}|n\rangle = \sqrt{n}|n-1\rangle$ and $\hat{c}^{\dagger}|n\rangle = \sqrt{n+1}|n+1\rangle$, the original Hamiltonian becomes [2]

$$\hat{\mathcal{H}}(\mathbf{k}) = \begin{pmatrix} m_- & 0 & \frac{\sqrt{2}v_\perp\hbar}{\ell_B}\sqrt{n} & v_z\hbar k_z \\ 0 & m_+ & v_z\hbar k_z & -\frac{\sqrt{2}v_\perp\hbar}{\ell_B}\sqrt{n} \\ \frac{\sqrt{2}v_\perp\hbar}{\ell_B}\sqrt{n} & v_z\hbar k_z & -m_+ & 0 \\ v_z\hbar k_z & -\frac{\sqrt{2}v_\perp\hbar}{\ell_B}\sqrt{n} & 0 & -m_- \end{pmatrix}, \tag{S5}$$

where

$$m_\pm = M_0 + \frac{M_\perp}{\ell_B^2}(2n \pm 1) + M_z k_z^2, \tag{S6}$$

$M_\perp = M_1 v_\perp^2$, $n \geqslant 0$ is the Landau level index, and it is an integer.

For $n \geqslant 1$, the energy eigenvalues of Eq. (S5) are

$$E^{(n)}_{k_z} = \begin{cases} \sqrt{(\hbar v_z k_z)^2 + m_+^2 + \frac{2nv_\perp^2\hbar^2}{\ell_B^2}}; \\ -\sqrt{(\hbar v_z k_z)^2 + m_+^2 + \frac{2nv_\perp^2\hbar^2}{\ell_B^2}}. \end{cases} \tag{S7}$$

## SII. QUANTUM LIMIT

In the quantum limit, only the 0th Landau level is occupied by the electrons, so we only focus on $n = 0$ case, the trial wave function becomes $(0, |0\rangle, |0\rangle, 0)^T$, the single-particle Hamiltonian density becomes

$$\hat{\mathcal{H}}^{(n=0)}(\mathbf{k}) = \begin{pmatrix} m_+ & v_z\hbar k_z \\ v_z\hbar k_z & -m_+ \end{pmatrix}, \tag{S8}$$

where $m_+ = M_0 + M_\perp/\ell_B^2 + M_z k_z^2$. Its energy eigenvalues are

$$E^{(0+)}_{k_z} = \mathrm{sgn}(m_+)\sqrt{(\hbar v_z k_z)^2 + m_+^2}, \tag{S9}$$

$$E^{(0-)}_{k_z} = -\mathrm{sgn}(m_+)\sqrt{(\hbar v_z k_z)^2 + m_+^2}. \tag{S10}$$

With $k_z = k_F$ in Eq. (S9), the Fermi energy is

$$E_F = E^{(0+)}_{k_z=k_F} = \sqrt{(\hbar v_z k_F)^2 + \left(M_0 + \frac{M_\perp}{\ell_B^2} + M_z k_F^2\right)^2}, \tag{S11}$$

where the Fermi wave vector along the $z$ direction is $k_F = 2\pi^2\hbar n_0/(eB)$ with the carrier density $n_0$.

With Eq. (S7) and $k_z = 0$, we can get the energy eigenvalue of $n = 1$ Landau level as [2]

$$E^{(1)}_{k_z=0} = \sqrt{\left(M_0 + \frac{3M_\perp}{\ell_B^2}\right)^2 + \frac{2v_\perp^2\hbar^2}{\ell_B^2}}. \tag{S12}$$

With $E^{(1)}_{k_z=0} = E_F$ and Eqs. (S11) and (S12), one can get the carrier density in the extreme quantum limit of the magnetic field $B = 1.3$ T [1] as $n_0 = 8.87 \times 10^{16}$ cm$^{-3}$.

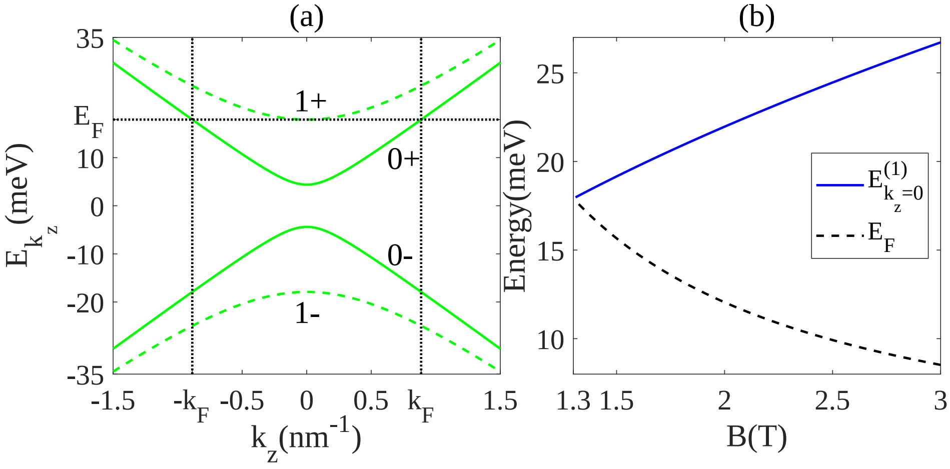


FIG. S1. (Color online) (a) $n = 0$ and $n = 1$ Landau levels without charge density wave (CDW) at the magnetic field $B = 1.3$ T where the Fermi energy touches the minimum of the $n = 1$ Landau level. (b) Fermi energy $E_F$ and $n = 1$ Landau level for $k_z = 0$ as functions of the magnetic field in the quantum limit. The parameters are set as as follows [1, 3]: $v_x = 9 \times 10^5$ m/s, $v_y = 1.9 \times 10^5$ m/s, $v_z = 0.3 \times 10^5$ m/s, $M_0 = -4.7$ meV, $M_\perp = 150$ meV·nm$^2$, $M_z = 0.01 M_\perp$, and $n_0 = 8.87 \times 10^{16}$ cm$^{-3}$.

Fig. S1(a) shows the dispersion of $n = 0$ and $n = 1$ Landau levels with magnetic field $B = 1.3$ T, where the Fermi energy touches the minimum of the $n = 1$ Landau level for noninteracting system. Solid lines and dashed green lines are for the $n = 0$ and $n = 1$ Landau levels, respectively. The dotted black transverse line is the Fermi energy $E_F$.

As shown in Fig. S1(b), we plot the Fermi energy $E_F$ and $n = 1$ Landau level for $k_z = 0$ as functions of the magnetic field in the quantum limit. The dashed black line is the Fermi energy and the solid blue line is the $n = 1$ Landau level for $k_z = 0$. It is found that the $n = 1$ Landau level for $k_z = 0$ is always higher than the Fermi energy in the quantum limit. It means that only the lowest 0+ Landau level is occupied in the quantum limit.

## SIII. LINEARIZATION

In order to obtain the effective Hamiltonian with electron-electron interactions, we need to get the linearization of the energy dispersion $E^{(0+)}_{k_z}$ of the single-particle Hamiltonian.

Similar to the linearization [5, 6], we can linearized the energy dispersion $E^{(0+)}_{k_z}$ of the lowest Landau level with small momentum $k_z$ near two Fermi wave vectors $\pm k_F \mathbf{e}_z$ as

$$E^{(0+)}_{k_z} = \begin{cases} v_F\hbar k_z, & \text{for } k_z \text{ near } k_F; \\ -v_F\hbar k_z, & \text{for } k_z \text{ near } -k_F, \end{cases} \tag{S13}$$

where the Fermi velocity along the $z$ direction is

$$v_F = \left|\frac{1}{\hbar}\frac{dE^{(0+)}_{k_z}}{dk_z}\Big|_{k_z=k_F}\right| = \left|\frac{(\hbar v_z)^2 k_F + 2m_F M_z k_F}{\hbar\sqrt{(\hbar v_z k_F)^2 + m_F^2}}\right|, \tag{S14}$$

$m_F = M_0 + M_\perp/\ell_B^2 + M_z k_F^2$, and $\mathbf{e}_z$ is the unit vector along $z$ direction.

In the basis of the eigenvector $\hat{\Psi}_\mathbf{k} = (\hat{d}_{\mathbf{k}+}, \hat{d}_{\mathbf{k}-})^{\mathrm{T}}$ for $E_{k_z}^{(0+)}$, the low-energy single-particle Hamiltonian density for $ZrTe_5$ is given by

$$\hat{\mathcal{H}}^{(n=0)}(\mathbf{k}) = \begin{pmatrix} v_F\hbar(k_z \pm k_F) & 0 \\ 0 & -v_F\hbar(k_z \pm k_F) \end{pmatrix}, \tag{S15}$$

where $\hat{d}^\dagger_{\mathbf{k}\pm}$ and $\hat{d}_{\mathbf{k}\pm}$ are the creation and annihilation operators in the vicinity of $\mp k_F$, and $\mathbf{k}\pm \equiv \mathbf{k} \pm k_F\mathbf{e}_z$.

## SIV. MEAN-FIELD APPROACH

The constraints for the accuracy of the mean-field approximation is determined by the fluctuations at finite temperatures [7, 8]. When the temperature approaches to or above the critical temperature (about 25 Kelvin in the experiment [1]) of the CDW state to normal state, the fluctuations become very important and the mean-field approximation fails. However, in the experiment [1], the measurements of the Hall and longitudinal resistivities are at 0.6 Kelvin, which is smallest compared to other energy scales, thus the fluctuations are sufficiently small and the accuracy of mean-field approximation can be justified.

In detail, the fluctuations on the length scales shorter than the correlation length are absorbed into the renormalized Landau parameters and do not produce deviations from the mean-field approximation [7]. This gives the precise formulation of the Ginzburg criterion which was first proposed by Levanyuk [9] and Ginzburg [10]. For mean-field theory to be reliable, the Ginzburg criterion is given as [7]

$$\frac{|T - T_C|}{T_C} \gg \left(\frac{k_B}{S_G}\right)^6, \tag{S16}$$

where $T$ is temperature, $T_C$ is the criticle temperature, $k_B$ is the Boltzmann constant, $S_G = \Delta C_V \xi_0$ in the dimensions of entropy with the specific heat jump $\Delta C_V = \pi^2 k_B^2 n(E_F) T_C/[7\zeta(3)]$ [5] and the zero-temperature coherence length $\xi_0 = \hbar v_F/(\pi|\Delta|)$ [5], $n(E_F) = N_L/(\pi\hbar v_F)$ is the density of states, $N_L = S_{xy}/(2\pi\ell_B^2)$ is the Landau degeneracy with the area $S_{xy} \sim (\mu \text{ m})^2$ in the $x - y$ plane. Therefore, one can have $k_B/S_G = 7\zeta(3)|\Delta|/(N_L k_B T_C)$. For $T = 0.6$ K and $T_C = 25$ K in the experiment [1], one can have $|T - T_C|/T_C = 0.976$.

As shown in Fig. S2, we calculate $(k_B/S_G)^6$ as a function of the magnetic field, and it is found that the Ginzburg criterion $(k_B/S_G)^6 \ll |T - T_C|/T_C$ is satisfied. Therefore, the mean-field approximation is justified.

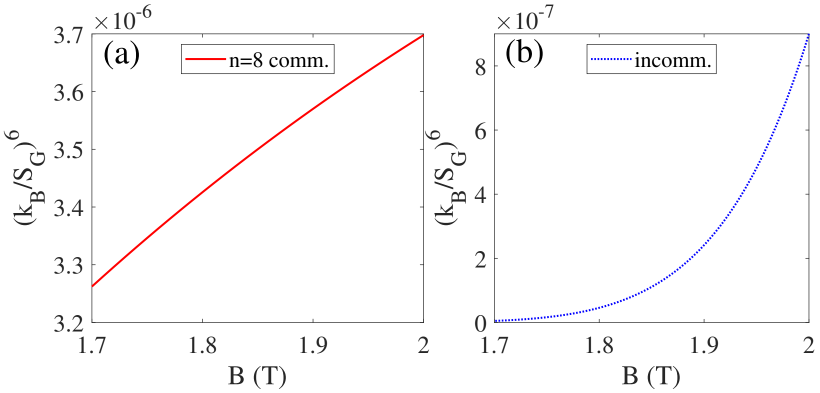


FIG. S2. (Color online) The Ginzburg criterion of the mean-field approach $(k_B/S_G)^6$ as a function of the magnetic field. (a) Commensurate case with $n = 8$. (b) Incommensurate case.

### A. Electron-electron interaction

The electron-electron interaction Hamiltonian can be written as [11–14]

$$\hat{H}_{ee} = \frac{1}{2}\sum_{\mathbf{k},\mathbf{k}',\mathbf{q}=\pm k_F\mathbf{e}_z} \frac{U(\mathbf{q})}{V} \hat{d}^\dagger_{\mathbf{k}+\mathbf{q}} \hat{d}^\dagger_{\mathbf{k}'-\mathbf{q}} \hat{d}_\mathbf{k} \hat{d}_{\mathbf{k}'} = \frac{1}{2}\sum_{\mathbf{k},\mathbf{k}',\mathbf{q}} \frac{U(\mathbf{q})}{V} \hat{d}^\dagger_{\mathbf{k}+\mathbf{q}} (\delta_{\mathbf{k}'-\mathbf{q},\mathbf{k}} - \hat{d}_\mathbf{k} \hat{d}^\dagger_{\mathbf{k}'-\mathbf{q}}) \hat{d}_{\mathbf{k}'}, \tag{S17}$$

where $U(\mathbf{q}) = e^2/[\epsilon(q^2+\kappa^2)]$ is the Yukawa potential, $1/\kappa$ is the Coulomb screening length, $\epsilon = \epsilon_r\epsilon_0$ is the dielectric constant with the relative dielectric constant $\epsilon_r$ and the permittivity of vacuum $\epsilon_0$, and $V$ is the volume. For simplicity, we set that $\mathbf{k}' - \mathbf{q} \neq \mathbf{k}$.

With the random phase approximation [Fig. 2 (b) in the main text], we have [11, 15]

$$\begin{aligned}
\kappa^2 &= \lim_{\omega_n\to 0, q\to 0} -\frac{e^2}{\epsilon}\frac{1}{2\pi\ell_B^2}\frac{1}{\beta}\sum_m \int_{-\infty}^{\infty}\frac{dk_z}{2\pi}\frac{1}{[i\hbar\omega_m - (E_{k_z}^{(0+)}-\mu)]}\frac{1}{[i\hbar(\omega_m+\omega_n) - (E_{k_z+q}^{(0+)}-\mu)]}\Bigg|_{T=0} \\
&= \lim_{\omega_n\to 0, q\to 0} -\frac{e^2}{\epsilon}\frac{eB}{2\pi\hbar}\int_{-\infty}^{\infty}\frac{dk_z}{2\pi}\frac{f(E_{k_z+q}^{(0+)}) - f(E_{k_z}^{(0+)})}{(E_{k_z+q}^{(0+)} - E_{k_z}^{(0+)}) - i\hbar\omega_n}\Bigg|_{T=0} \\
&\approx \lim_{\omega_n\to 0, q\to 0} -\frac{e^2}{\epsilon}\frac{eB}{2\pi\hbar}\int_{-\infty}^{\infty}\frac{dk_z}{2\pi}\frac{(E_{k_z+q}^{(0+)} - E_{k_z}^{(0+)})\frac{\partial f(E_{k_z}^{(0+)})}{\partial E_{k_z}^{(0+)}}}{(E_{k_z+q}^{(0+)} - E_{k_z}^{(0+)})}\Bigg|_{T=0} \\
&= -\frac{e^3 B}{4\pi^2\epsilon\hbar^2 v_F}\int_1^0 df(E_{k_z}^{(0+)})\Bigg|_{T=0} \\
&= \frac{e^3 B}{4\pi^2\epsilon\hbar^2 v_F},
\end{aligned} \tag{S18}$$

where $f(x) = 1/[1+e^{x/(k_B T)}]$ is the Fermi function and we use the summation of the fermion Matsubara frequencies $\omega_m$

$$\lim_{\eta\to 0}\sum_m \frac{e^{i\omega_m\eta}}{i\hbar\omega_m - x} = \frac{\beta}{e^{\beta x}+1}, \tag{S19}$$

$$\sum_m \frac{1}{(i\hbar\omega_m - \xi_k)[i\hbar(\omega_m+\omega_n) - \xi_{k+q}]} = \frac{f(\xi_k) - f(\xi_{k+q})}{i\hbar\omega_m + \xi_k - \xi_{k+q}}. \tag{S20}$$

For $\mathbf{q} = \pm 2k_F\mathbf{e}_z$, the mean-field electron-electron interaction Hamiltonian for CDW state is

$$\hat{H}_{ee} = -\sum_{\mathbf{k}} |\Delta| \left(e^{i\phi}\hat{d}^\dagger_{\mathbf{k}+}\hat{d}_{\mathbf{k}-} + e^{-i\phi}\hat{d}^\dagger_{\mathbf{k}-}\hat{d}_{\mathbf{k}+}\right) + \frac{2|\Delta|^2 V}{U(2k_F)}, \tag{S21}$$

where the order parameter is defined as $\Delta = |\Delta_{ee}|e^{i\phi} = [U(2k_F)/(2V)]\sum_{\mathbf{k}}\langle \hat{d}^\dagger_{\mathbf{k}-2k_F\mathbf{e}_z}\hat{d}_{\mathbf{k}}\rangle$, and $\phi$ is the phase of the order parameter.

In the basis $\hat{\Psi}_{\mathbf{k}} = (\hat{d}_{\mathbf{k}+}, \hat{d}_{\mathbf{k}-})^{\mathrm{T}}$, the effective Hamiltonian density becomes

$$\hat{\mathcal{H}}^{0+}_{k_z} = \hat{\mathcal{H}}^{(n=0)}(\mathbf{k}) + \hat{\mathcal{H}}_{ee}(\mathbf{k}) = \begin{pmatrix} v_F\hbar(k_z \pm k_F) & |\Delta|e^{i(\phi+\pi)} \\ |\Delta|e^{i(-\phi+\pi)} & -v_F\hbar(k_z\pm k_F)\end{pmatrix}, \tag{S22}$$

where $\hat{\mathcal{H}}_{ee}(\mathbf{k}) = -|\Delta|\left(e^{i\phi}\hat{d}^\dagger_{\mathbf{k}+}\hat{d}_{\mathbf{k}-} + e^{-i\phi}\hat{d}^\dagger_{\mathbf{k}-}\hat{d}_{\mathbf{k}+}\right)$ is the density of the mean-field electron-electron interaction Hamiltonian.

Therefore, the CDW energy eigenvalues near the Fermi surface are given by

$$E_{k_z} = E_F + \mathrm{sgn}(k_z - k_F)\sqrt{[v_F\hbar(k_z-k_F)]^2 + |\Delta|^2}, \text{ for } k_z \text{ near } k_F; \tag{S23}$$

$$E_{k_z} = E_F - \mathrm{sgn}(k_z + k_F)\sqrt{[v_F\hbar(k_z+k_F)]^2 + |\Delta|^2}, \text{ for } k_z \text{ near } -k_F, \tag{S24}$$

where $\mathrm{sgn}(x)$ is the signum function.

### B. Electron-phonon interaction

The electron-phonon interaction Hamiltonian can be written as [5, 11, 16, 17]

$$\hat{H}_{e-ph} = \sum_{\mathbf{k},\mathbf{q}}\frac{\alpha_{\mathbf{q}}}{V}\hat{d}^\dagger_{\mathbf{k}+\mathbf{q}}\hat{d}_{\mathbf{k}}(\hat{b}^\dagger_{-\mathbf{q}} + \hat{b}_{\mathbf{q}}), \tag{S25}$$

where $\hat{b}^\dagger_{\mathbf{q}}$ and $\hat{b}_{\mathbf{q}}$ are the creation and annihilation operators for the phonons with momentum $\mathbf{q}$, the phonon dispersion is given by $\omega_{\mathbf{q}} = v_s q$ with the velocity of sound $v_s$, the electron-phonon coupling is [11] $\alpha_{\mathbf{q}} = -iqV_{\mathbf{q}}\sqrt{N_{\text{ion}}\hbar/(2M\omega_{\mathbf{q}})}$ in the isotropic case for normal acoustical phonon, $V_{\mathbf{q}} = -Ze^2/[\epsilon(q^2+\kappa^2)]$ is the Yukawa potential, $Ze$ is the ionic charge, $M$ is the ionic mass, $N_{\text{ion}}$ is the ionic number, and $V$ is the volume.

For $\mathbf{q} = \pm 2k_F\mathbf{e}_z$, the mean-field electron-phonon interaction Hamiltonian for CDW state is

$$\hat{H}_{e-ph} = \sum_{\mathbf{k}} |\Delta| \left(e^{i\phi}\hat{d}^\dagger_{\mathbf{k}+}\hat{d}_{\mathbf{k}-} + e^{-i\phi}\hat{d}^\dagger_{\mathbf{k}-}\hat{d}_{\mathbf{k}+}\right), \tag{S26}$$

where the order parameter is defined as $\Delta = |\Delta_{e-ph}|e^{i\phi} \equiv (\alpha_{2k_F}/V)(\langle\hat{b}^\dagger_{-2k_F\mathbf{e}_z}\rangle + \langle\hat{b}_{2k_F\mathbf{e}_z}\rangle)$, and $\phi$ is the phase of the order parameter.

The Hamiltonian for the phonons is given by

$$\hat{H}_{ph} = \sum_{\mathbf{q}} \hbar\omega_{\mathbf{q}}\hat{b}^\dagger_{\mathbf{q}}\hat{b}_{\mathbf{q}}. \tag{S27}$$

Further, the mean-field Hamiltonian for the phonons is given by

$$\hat{H}_{ph} = 2\hbar\omega_{2k_F}\langle\hat{b}_{2k_F}\rangle^2 = \frac{\hbar\omega_{2k_F}|\Delta|^2V}{2|\alpha_{2k_F}|^2} = \frac{Mv_s^2|\Delta|^2V}{N_{\text{ion}}V^2_{2k_F}} = \frac{Mv_s^2\epsilon^2[(2k_F)^2+\kappa^2]^2|\Delta|^2V}{N_{\text{ion}}Z^2e^4}, \tag{S28}$$

where we set that $\langle\hat{b}^\dagger_{-2k_F}\rangle = \langle\hat{b}_{2k_F}\rangle$.

In the basis $\hat{\Psi}_{\mathbf{k}} = (\hat{d}_{\mathbf{k}+}, \hat{d}_{\mathbf{k}-})^{\text{T}}$, the effective Hamiltonian density becomes

$$\hat{\mathcal{H}}^{0+}_{k_z} = \hat{\mathcal{H}}^{(n=0)}(\mathbf{k}) + \hat{\mathcal{H}}_{e-ph}(\mathbf{k}) = \begin{pmatrix} v_F\hbar(k_z \pm k_F) & |\Delta|e^{i\phi} \\ |\Delta|e^{-i\phi} & -v_F\hbar(k_z \pm k_F) \end{pmatrix}, \tag{S29}$$

where $\hat{\mathcal{H}}_{e-ph}(\mathbf{k}) = |\Delta|\left(e^{i\phi}\hat{d}^\dagger_{\mathbf{k}+}\hat{d}_{\mathbf{k}-} + e^{-i\phi}\hat{d}^\dagger_{\mathbf{k}-}\hat{d}_{\mathbf{k}+}\right)$ is the density of the mean-field electron-phonon interaction Hamiltonian.

Therefore, the CDW energy eigenvalues near the Fermi surface are given by

$$E_{k_z} = E_F + \text{sgn}(k_z - k_F)\sqrt{[v_F\hbar(k_z-k_F)]^2 + |\Delta|^2}, \text{ for } k_z \text{ near } k_F; \tag{S30}$$

$$E_{k_z} = E_F - \text{sgn}(k_z + k_F)\sqrt{[v_F\hbar(k_z+k_F)]^2 + |\Delta|^2}, \text{ for } k_z \text{ near } -k_F, \tag{S31}$$

where $\text{sgn}(x)$ is the signum function.

## SV. GROUND-STATE ENERGY AND PERIOD OF THE CDW STATE

With Eqs. (S22) and (S29), the mean-field effective Hamiltonian of the lowest 0+ Landau band for $ZrTe_5$ in the basis $\hat{\Psi}_{\mathbf{k}} = (\hat{d}_{\mathbf{k}+}, \hat{d}_{\mathbf{k}-})^{\text{T}}$ is given by

$$\hat{H}_m = \sum_{\mathbf{k}} \hat{\Psi}^\dagger_{\mathbf{k}}\hat{\mathcal{H}}^{0+}_{k_z}\hat{\Psi}_{\mathbf{k}} + \frac{|\Delta|^2V}{g_{2k_F}}, \tag{S32}$$

where $g_{2k_F} = e^2/\{2\epsilon[(2k_F)^2+\kappa^2]\}$ with $\kappa = \sqrt{e^3B/(4\pi^2\epsilon\hbar^2v_F)}$ for electron-electron interactions and $g_{2k_F} = g_0/[(2k_F)^2+\kappa^2]^2$ for electron-phonon interactions with $g_0 = N_{\text{ion}}Z^2e^4/(Mv_s^2\epsilon^2)$.

In the following derivations, we take the electron-phonon case [Eq. (S29)] as an exmaple to get the ground-state energy and periodic charge density variation. We define a new set of operators by [5]

$$\hat{\gamma}_{\mathbf{k},1} = U_{\mathbf{k}}e^{-i\phi/2}\hat{d}_{\mathbf{k}+} - V_{\mathbf{k}}e^{i\phi/2}\hat{d}_{\mathbf{k}-}, \tag{S33}$$

$$\hat{\gamma}_{\mathbf{k},2} = V_{\mathbf{k}}e^{-i\phi/2}\hat{d}_{\mathbf{k}+} + U_{\mathbf{k}}e^{i\phi/2}\hat{d}_{\mathbf{k}-}. \tag{S34}$$

Further, the effective Hamiltonian density $\hat{\Psi}^\dagger_{\mathbf{k}}\hat{\mathcal{H}}^{0+}_{k_z}\hat{\Psi}_{\mathbf{k}}$ in Eq. (S32) can be written in terms of $\hat{\gamma}_{\mathbf{k},1}$ and $\hat{\gamma}_{\mathbf{k},2}$ as

$$\begin{aligned}\hat{\Psi}^\dagger_{\mathbf{k}}\hat{\mathcal{H}}^{0+}_{k_z}\hat{\Psi}_{\mathbf{k}} &= E^{(0)}_{k_z}\left(\hat{d}^\dagger_{\mathbf{k}+}\hat{d}_{\mathbf{k}+} - \hat{d}^\dagger_{\mathbf{k}-}\hat{d}_{\mathbf{k}-}\right) + |\Delta|\left(e^{i\phi}\hat{d}^\dagger_{\mathbf{k}+}\hat{d}_{\mathbf{k}-} + e^{-i\phi}\hat{d}^\dagger_{\mathbf{k}-}\hat{d}_{\mathbf{k}+}\right) \\ &= \left[E^{(0)}_{k_z}(U^2_{\mathbf{k}} - V^2_{\mathbf{k}}) - 2|\Delta|U_{\mathbf{k}}V_{\mathbf{k}}\right](\hat{\gamma}^\dagger_{\mathbf{k},1}\hat{\gamma}_{\mathbf{k},1} - \hat{\gamma}^\dagger_{\mathbf{k},2}\hat{\gamma}_{\mathbf{k},2}) \\ &\quad + \left[|\Delta|(U^2_{\mathbf{k}} - V^2_{\mathbf{k}}) + 2E^{(0)}_{k_z}U_{\mathbf{k}}V_{\mathbf{k}}\right](\hat{\gamma}^\dagger_{\mathbf{k},1}\hat{\gamma}_{\mathbf{k},2} + \hat{\gamma}^\dagger_{\mathbf{k},2}\hat{\gamma}_{\mathbf{k},1}),\end{aligned} \tag{S35}$$

where $E_{k_z}^{(0)} = v_F \hbar (k_z \pm k_F)$ near $\mp k_F$.

The Hamiltonian density is diagonalized if the coefficients in front of the off-diagonal terms are zero, i.e.,

$$|\Delta|(U_{\mathbf{k}}^2 - V_{\mathbf{k}}^2) + 2E_{k_z}^{(0)} U_{\mathbf{k}} V_{\mathbf{k}} = 0. \tag{S36}$$

The condition $U_{\mathbf{k}}^2 + V_{\mathbf{k}}^2 = 1$ is satisfied if we choose

$$U_{\mathbf{k}}^2 = \frac{1}{2}\left(1 + \frac{E_{k_z}^{(0)}}{\sqrt{(E_{k_z}^{(0)})^2 + |\Delta|^2}}\right), \tag{S37}$$

$$V_{\mathbf{k}}^2 = \frac{1}{2}\left(1 - \frac{E_{k_z}^{(0)}}{\sqrt{(E_{k_z}^{(0)})^2 + |\Delta|^2}}\right). \tag{S38}$$

Therefore, the effective Hamiltonian density (S35) becomes [5]

$$\hat{\Psi}_{\mathbf{k}}^\dagger \hat{\mathcal{H}}_{k_z}^{0+} \hat{\Psi}_{\mathbf{k}} = E_{k_z}(\hat{\gamma}_{\mathbf{k},1}^\dagger \hat{\gamma}_{\mathbf{k},1} + \hat{\gamma}_{\mathbf{k},2}^\dagger \hat{\gamma}_{\mathbf{k},2}), \tag{S39}$$

where we have used $U_{\mathbf{k}} V_{\mathbf{k}} < 0$, $E_{k_z}$ are the CDW eigenvalues of $\hat{\mathcal{H}}_{k_z}^{0+}$ in Eq. (S29), and

$$E_{k_z} = E_F \pm \mathrm{sgn}(k_z \mp k_F)\sqrt{[v_F \hbar (k_z \mp k_F)]^2 + |\Delta|^2}, \text{ for } k_z \text{ near } \pm k_F. \tag{S40}$$

The ground-state wave function is given by [5]

$$|\Phi_0\rangle = \left(\prod_{k_z < k_F} \hat{\gamma}_{\mathbf{k},1}^\dagger \hat{\gamma}_{\mathbf{k},2}^\dagger\right)|0\rangle, \tag{S41}$$

$|0\rangle$ represents the vacuum state.

Therefore, the ground-state energy solution can be obtained by minimizing

$$E_g = \langle \Phi_0 | \hat{H}_m | \Phi_0 \rangle = \sum_{\mathbf{k}} (E_{k_z} - E_F)\Theta\left(E_F - E_{k_z}\right) + \frac{|\Delta|^2 V}{g_{2k_F}}, \tag{S42}$$

where $\hat{H}_m = \sum_{\mathbf{k}} E_{k_z}(\hat{\gamma}_{\mathbf{k},1}^\dagger \hat{\gamma}_{\mathbf{k},1} + \hat{\gamma}_{\mathbf{k},2}^\dagger \hat{\gamma}_{\mathbf{k},2}) + |\Delta|^2 V / g_{2k_F}$ is the mean-field effective Hamiltonian, $\Theta(x)$ is the step function, and we have used

$$\langle \Phi_0 | \hat{\gamma}_{\mathbf{k},1}^\dagger \hat{\gamma}_{\mathbf{k},1} | \Phi_0 \rangle = \langle \Phi_0 | \hat{\gamma}_{\mathbf{k},2}^\dagger \hat{\gamma}_{\mathbf{k},2} | \Phi_0 \rangle = 1, \tag{S43}$$

$$\langle \Phi_0 | \hat{\gamma}_{\mathbf{k},1}^\dagger \hat{\gamma}_{\mathbf{k},2} | \Phi_0 \rangle = \langle \Phi_0 | \hat{\gamma}_{\mathbf{k},2}^\dagger \hat{\gamma}_{\mathbf{k},1} | \Phi_0 \rangle = 0. \tag{S44}$$

Meanwhile, the electronic density is given by [5]

$$\rho(z) = \langle \Phi_0 | \hat{\Psi}^\dagger(z) \hat{\Psi}(z) | \Phi_0 \rangle = \sum_{\mathbf{k}} \left[1 + \frac{|\Delta|}{\sqrt{(E_{k_z}^{(0)})^2 + |\Delta|^2}} \cos(2k_F z + \phi)\right], \tag{S45}$$

where $\hat{\Psi}(z) = \sum_{\mathbf{k}} \left(\hat{d}_{\mathbf{k}+} e^{ik_F z} + \hat{d}_{\mathbf{k}-} e^{-ik_F z}\right)$.

With Eq. (S45), we can get the periodic wave length of the CDW state as

$$\lambda_{cdw} = \frac{2\pi}{2k_F} = \frac{1}{2}\lambda_F, \tag{S46}$$

which is consistent with the experiment [1] (the Figure 3 (b) of Ref. [1]). Here, $\lambda_F = 2\pi/k_F$ is the Fermi wave length.

## SVI. GAP EQUATION

### A. Density of state for CDW

With the CDW energy eigenvalues near the Fermi surface given by Eqs. (S30) and (S31), one can obtain

$$\frac{\partial E_{k_z}}{\partial k_z} = \frac{\mathrm{sgn}(k_z - k_F) v_F^2 \hbar^2 |k_z - k_F|}{\sqrt{[v_F \hbar (k_z - k_F)]^2 + |\Delta|^2}}, \text{ for } k_z \text{ near } k_F; \tag{S47}$$

$$\frac{\partial E_{k_z}}{\partial k_z} = \frac{-\mathrm{sgn}(k_z + k_F) v_F^2 \hbar^2 |k_z + k_F|}{\sqrt{[v_F \hbar (k_z + k_F)]^2 + |\Delta|^2}}, \text{ for } k_z \text{ near } -k_F. \tag{S48}$$

Further, we can get

$$\frac{\partial E_{k_z}}{\partial k_z} = \frac{v_F \hbar \sqrt{(E_{k_z} - E_F)^2 - |\Delta|^2}}{E_{k_z} - E_F}. \tag{S49}$$

Then, the density of states along the $z$ direction is given by

$$D_z(E_{k_z}) = \frac{L_z}{2\pi} \left| \frac{\partial k_z}{\partial E_{k_z}} \right| = \begin{cases} \frac{L_z |E_{k_z} - E_F|}{2\pi v_F \hbar \sqrt{(E_{k_z} - E_F)^2 - |\Delta|^2}}, & E_{\mathrm{min}} < E_{k_z} < E_{\mathrm{max}}; \\ 0, & \text{other regions,} \end{cases} \tag{S50}$$

where $L_z$ is the length along the $z$ direction, $E_{\mathrm{min}} = E_F - \sqrt{(v_F \hbar k_F)^2 + |\Delta|^2}$, and $E_{\mathrm{max}} = E_F - |\Delta|$.

The summations over $k_x$ and $k_y$ just give the Landau degeneracy $\sum_{k_x, k_y} = N_L = S_{xy}/(2\pi \ell_B^2)$ with the area $S_{xy}$ in the $x - y$ plane.

Therefore, the total CDW density of states is given by

$$D_{cdw}(E_{k_z}) = N_L D_z(E_{k_z}) = \begin{cases} \frac{V}{(2\pi)^2 \ell_B^2 v_F \hbar} \frac{|E_{k_z} - E_F|}{\sqrt{(E_{k_z} - E_F)^2 - |\Delta|^2}}, & E_{\mathrm{min}} < E_{k_z} < E_{\mathrm{max}}; \\ 0, & \text{other regions,} \end{cases} \tag{S51}$$

where we set that $V = S_{xy} L_z$.

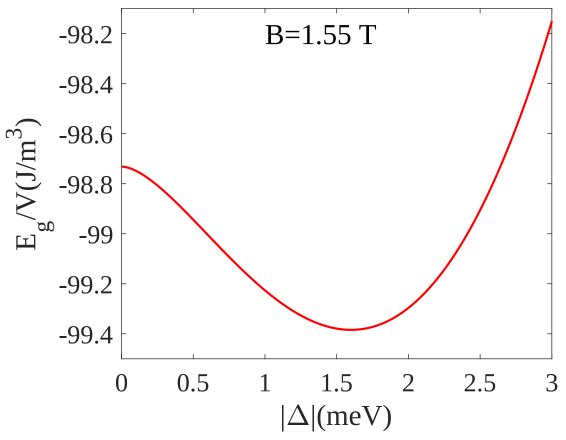


FIG. S3. (Color online) The ground-state energy as a function of the order parameter at $B = 1.55$ T.

### B. Zero-temperature case

Substituting Eq. (S51) into (S42), we have the ground-state energy as

$$E_g = -\frac{VeB}{2\pi^2 v_F \hbar^2} \int_0^{v_F \hbar k_F} \sqrt{t_{k_z}^2 + |\Delta|^2} dt_{k_z} + \frac{|\Delta|^2 V}{g_{2k_F}} \tag{S52}$$

$$= -\frac{VeB}{4\pi^2 v_F \hbar^2} \left[ v_F \hbar k_F \sqrt{(v_F \hbar k_F)^2 + \Delta^2} - |\Delta|^2 \ln |\Delta| + |\Delta|^2 \ln(v_F \hbar k_F + \sqrt{(v_F \hbar k_F)^2 + \Delta^2}) \right] + \frac{|\Delta|^2 V}{g_{2k_F}}, \tag{S53}$$

where $t_{k_z} = \sqrt{\xi_{k_z}^2 - |\Delta|^2}$, $\xi_{k_z} = E_{k_z} - E_F$, and $E_{k_z}$ are the CDW eigenvalues of $\hat{\mathcal{H}}_{k_z}^{0+}$ in Eq. (S29).

In order to minimize the above ground-state energy Eq. (S52), we have the gap equation as $\partial E_g/\partial|\Delta| = 0$, i.e.,

$$\int_0^{v_F\hbar k_F} \frac{dt_{k_z}}{\sqrt{t_{k_z}^2 + |\Delta|^2}} = \frac{4\pi^2\hbar^2 v_F}{g_{2k_F} eB}. \tag{S54}$$

Further, the gap equation can be reduced to

$$|\Delta| = \left|(v_F\hbar k_F)\,\mathrm{csch}\left(\frac{4\pi^2\hbar^2 v_F}{g_{2k_F} eB}\right)\right|. \tag{S55}$$

We plot the ground-state energy as a function of the order parameter at $B = 1.55$ T in Fig. S3 to show that the solution of the gap equation (S55) can be used to minimize the ground-state energy.

### C. Finite-temperature case

The finite-temperature thermodynamic potential is given by [18]

$$\begin{aligned}\Omega &= -k_B T \ln \mathrm{Tr} e^{-\hat{H}_\mu/(k_B T)} \\ &\simeq -k_B T \sum_{\mathbf{k}} \ln\left[1 + e^{-E(k_z,\mu)/(k_B T)}\right] + \frac{1}{2}\sum_{\mathbf{q}=\pm 2\mu/(v_F\hbar)} \frac{|\Delta|^2 V}{g_{\mathbf{q}}} \\ &= -\frac{VeBk_BT}{2\pi^2 v_F\hbar^2}\int_0^\mu \ln\left[1 + e^{E_T(t,\Delta)/(k_BT)}\right] dt + \frac{1}{2}\sum_{\mathbf{q}=\pm 2\mu/(v_F\hbar)} \frac{|\Delta|^2 V}{g_{\mathbf{q}}},\end{aligned} \tag{S56}$$

where we use very low temperature as an approximation,

$$\hat{H}_\mu = \sum_{\mathbf{k}} \hat{\Psi}_{\mathbf{k}}^\dagger \hat{\mathcal{H}}_\mu \hat{\Psi}_{\mathbf{k}} + \frac{1}{2}\sum_{\mathbf{q}=\pm 2\mu/(v_F\hbar)} \frac{|\Delta|^2 V}{g_{\mathbf{q}}}, \tag{S57}$$

$$\hat{\mathcal{H}}_\mu = \begin{pmatrix} v_F\hbar k_z \pm \mu & |\Delta|e^{i\phi} \\ |\Delta|e^{-i\phi} & -(v_F\hbar k_z \pm \mu) \end{pmatrix}, \tag{S58}$$

$\mu$ is the chemical potential, $k_B$ is the Boltzmann constant, $T$ is the temperature, $E(k_z,\mu) = \pm\mathrm{sgn}(v_F\hbar k_z \mp \mu)\sqrt{(v_F\hbar k_z \mp \mu)^2 + |\Delta|^2}$ with $k_z$ near $\pm\mu/(v_F\hbar)$, $E_T(t,\Delta) = \sqrt{t^2 + |\Delta|^2}$, $t = \sqrt{\xi^2 - |\Delta|^2}$, and $\xi = v_F\hbar k_z - \mu$.

The finite-temperature gap equation is given by $\partial\Omega/\partial|\Delta| = 0$, i.e.,

$$\int_0^\mu \frac{1}{1 + e^{-\beta E_T(t,\Delta)}} \frac{dt}{E_T(t,\Delta)} = \frac{1}{2}\sum_{\mathbf{q}=\pm\mu/(v_F\hbar)} \frac{4\pi^2\hbar^2 v_F}{g_{\mathbf{q}} eB}. \tag{S59}$$

For extrmely low temperature, i.e., $T \to 0$, we have $\mu \to v_F\hbar k_F$. Further, the finite-temperature gap equation can be reduced to

$$\int_0^{v_F\hbar k_F} \frac{1}{1 + e^{-E_T(t,\Delta)/(k_BT)}} \frac{dt}{E_T(t,\Delta)} = \frac{4\pi^2\hbar^2 v_F}{g_{2k_F} eB}. \tag{S60}$$

As shown in Table. S1, we calculate the finite-temperature order parameters for $T = 0, 1.5, 2, 2.5$ K.

| T (K) | 0 | 1.5 | 2.0 | 2.5 |
|---|---|---|---|---|
| $\|\Delta\|$ (meV) | 1.6000092 | 1.6000055 | 1.5999471 | 1.5995734 |

TABLE S1. Table of order parameters for different temperatures at $B = 1.55$ T.

## SVII. LATTICE IONIC POTENTIAL ENERGY

The ground-state energy of the commensurate phase requires further information regarding the ionic potential of the crystal. The locking potential describing the interaction of the CDW with the underlying crystal lattice can be written as [5, 19]

$$V_{\text{lock}} = \rho_0 V_0 [1 - \cos(M\phi)], \tag{S61}$$

where $M = \lambda_{cdw}/a$ is the degree of commensurability, $\rho_0$ is the amplitude of the CDW, and $\phi$ is the phase variable. The potential $\rho_0 V_0$ can be derived from a microscopic theory using weak coupling arguments and it decreases with an increasing degree of commensurability $M$.

As will be discussed, for such higher order commensurability the potential $V_0$ is small, and consequently the energy associated with the periodic variation of the phase is also small and can be easily overshadowed by other effects such as interactions with impurity potentials [5].

For a commensurability $M$, one obtains the lattice ionic potential energy or commensurability energy as [5, 20]

$$E_{\text{comm}} = -\frac{|\Delta|^2 V}{g_{2k_F}} \left(\frac{|\Delta|}{D}\right)^{M-2} \cos(M\phi), \tag{S62}$$

where $\Delta$ is complex and its phase $\phi$ determines the relative position of the CDW and the lattice, $D$ is a cutoff energy, assumed to be on the order of the bandwidth [5, 20]. Here, we choose $D = |2t_z|$ with the hopping $t_z = -0.0679$ eV along the $z$ direction [1].

Within the mean-field approximation, the fluctuations of the amplitude and phase of the order parameter are not included in the following calculations. Therefore, the ground-state energy in commensurate state can be obtained by minimizing

$$\begin{aligned}
E_g &= \sum_{\mathbf{k}} (E_{k_z} - E_F)\Theta(E_F - E_{k_z}) + \frac{|\Delta|^2 V}{g_{2k_F}} + E_{\text{comm}} \\
&= -\frac{VeB}{2\pi^2 v_F \hbar^2} \int_0^{v_F\hbar k_F} \sqrt{t_{k_z}^2 + |\Delta|^2} dt_{k_z} + \frac{|\Delta|^2 V}{g_{2k_F}} \left[1 - \left(\frac{|\Delta|}{D}\right)^{M-2} \cos(M\phi)\right] \\
&= -\frac{VeB}{4\pi^2 v_F \hbar^2} \left[v_F\hbar k_F \sqrt{(v_F\hbar k_F)^2 + \Delta^2} - |\Delta|^2 \ln|\Delta| + |\Delta|^2 \ln(v_F\hbar k_F + \sqrt{(v_F\hbar k_F)^2 + \Delta^2})\right] \\
&\quad + \frac{|\Delta|^2 V}{g_{2k_F}} \left[1 - \left(\frac{|\Delta|}{D}\right)^{M-2} \cos(M\phi)\right],
\end{aligned} \tag{S63}$$

where we use the density of state for CDW, i.e., Eq. (S51).

By setting $M = 8$ and $\phi = 0.01$, we have the lattice ionic potential energy or commensurability energy as

$$E_{\text{comm}} = -\frac{|\Delta|^2 V}{g_{2k_F}} \left(\frac{|\Delta|}{D}\right)^6 \cos(0.08). \tag{S64}$$

As show in Fig. S4 Left, compared with the ground-state energy, the commensurability energy is too small to be included numerically.

We also plot the ground-state energies (per unit volume) of the commensurate ($\lambda_{cdw}/a = 8$) CDWs with and without the commensurability energy as shown in Fig. S4 Right. It is found that the two ground-state energies almost overlap with each other.

## SVIII. TUNNELING CURRENT ALONG THE DIRECTION OF MAGNETIC FIELD

### A. Density of states

In order to calculate the electric current, differential conductance and resistance, we need to get the density of sates. The density of states in the CDW state is obtained from the condition

$$D_{cdw}(E_{k_z}) dE_{k_z} = D_N(\epsilon_{k_z}) d\epsilon_{k_z}, \tag{S65}$$

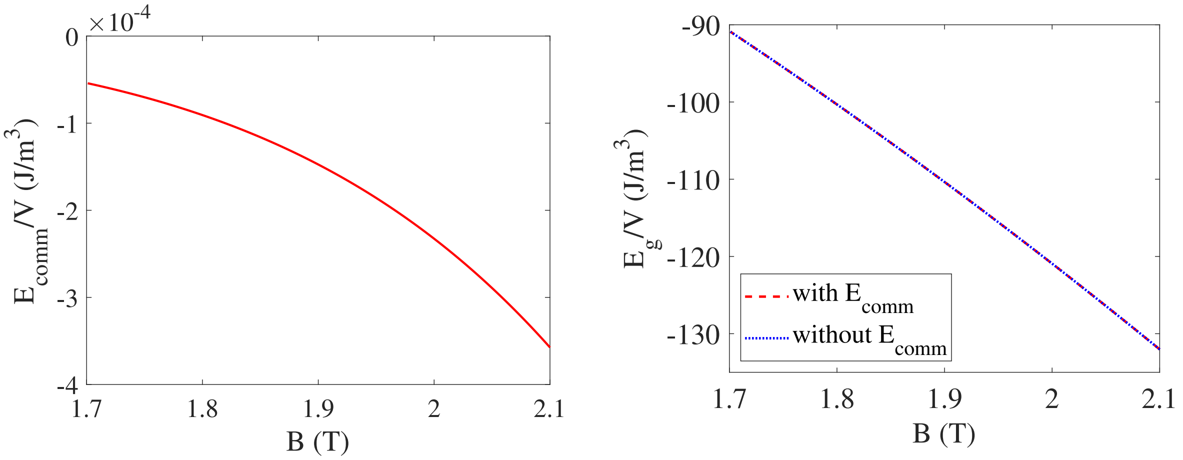


FIG. S4. (Color online) Left: The lattice ionic potential energy or commensurability energy (per unit volume) as a function of the magnetic field. Here, $M = 8$ and $\phi = 0.01$. Right: The ground-state energies $E_g$ (per unit volume) of the commensurate ($\lambda_{cdw}/a = 8$) CDWs. The red dashed curve represents $E_g$ with the commensurability energy and the blue dotted curve represents the one without the commensurability energy.

where $\epsilon_{k_z} = v_F \hbar k_z$.

Assuming that the density of states in the metallic state of the electrode "$N$", $D_N(\epsilon_{k_z}) = D_N(0)$ is assumed to be independent of the energy near the Fermi surface, we have

$$\frac{D_{cdw}(E_{k_z})}{D_N(0)} = \left|\frac{d\epsilon_{k_z}}{dE_{k_z}}\right| = \begin{cases} 0, & |E_{k_z} - E_F| < |\Delta|; \\ \frac{|E_{k_z}-E_F|}{\sqrt{(E_{k_z}-E_F)^2 - |\Delta|^2}}, & |E_{k_z} - E_F| > |\Delta|. \end{cases} \tag{S66}$$

### B. Non-Ohmic character along the $z$-direction

In order to compare with the experimental data and determine the value of the electron-phonon coupling constant $g_0$, we calculate the tunneling current and differential resistance as follows.

Different from Bardeen's phenomenological tunneling model [21, 22], we calculate the current-voltage characteristics based on the density of states Eq. (S66).

With the normal metals "$N1$" and "$N2$" represented by an energy independent density of states $D_{N1}(0)$ and $D_{N2}(0)$, respectively, the zero-temperature tunneling current is given by [5, 23]

$$I_{cdw}(V_z) = \frac{e}{h}|\mathcal{T}|^2 \int_{-\infty}^{\infty} d\epsilon \; D_{cdw}(\epsilon) D_{N2}(\epsilon + eV_z) = G_{cdw}^{(i)} V_{\text{eff}}, \tag{S67}$$

where $\mathcal{T}$ is the tunneling matrix element which is assumed energy-independent and can be approximated as a constant, $V_{\text{eff}} = \sqrt{[(eV_z)^2 - |\Delta|^2]/e^2}$ is the effective voltage, $G_{cdw}^{(i)} = e^2|\mathcal{T}|^2 D_{N1}(0) D_{N2}(0)/h$ is the conductance for the CDW state with $i = 1, 2, 3$, and $V_z$ is the longitudinal voltage along the $z$-direction.

There is no tunneling current as long as $e|V_z| < |\Delta|$. Therefore, we can define the threshold voltage as $V_{th} = |\Delta|/e$. However, for nonzero temperatures, a small tunneling current is expected even for voltages less than the single particle gap $|\Delta|$.

The zero-temperature differential conductance is given by [5, 23]

$$G_{cdw}(V_z) = \left(\frac{dI_{cdw}}{dV_z}\right)_{T=0} = G_{cdw}^{(i)} \frac{|eV_z|}{\sqrt{(eV_z)^2 - |\Delta|^2}}. \tag{S68}$$

At finite temperatures, the tunneling current is given by [5, 23]

$$I_{cdw}(V_z) = \frac{e}{h}|\mathcal{T}|^2 \int_{-\infty}^{\infty} d\epsilon \; D_{cdw}(\epsilon) D_{N2}(\epsilon + eV_z)[f(\epsilon) - f(\epsilon + eV_z)] = G_{cdw}^{(i)} \int_{-\infty}^{\infty} d\epsilon \; \frac{|\epsilon|[f(\epsilon) - f(\epsilon + eV_z)]}{e\sqrt{\epsilon^2 - |\Delta|^2}}, \tag{S69}$$

where $f(x) = 1/[1 + e^{x/(k_B T)}]$ is the Fermi function [18].

The corresponding finite-temperature differential conductance is given by [5, 23]

$$G_{cdw}(V_z) = \frac{dI_{cdw}}{dV_z} = G_{cdw}^{(i)} \int_{-\infty}^{\infty} d\epsilon \, \frac{|\epsilon|}{\sqrt{\epsilon^2 - |\Delta|^2}} \frac{\beta \exp[\beta(\epsilon + eV_z)]}{\{1 + \exp[\beta(\epsilon + eV_z)]\}^2}, \tag{S70}$$

where $\beta = 1/(k_B T)$.

When $ZrTe_5$ becomes a metal with the density of states $D_{N0}(0)$, the tunneling current between two normal metals is given by [23]

$$I_N(V_z) = \frac{e}{h}|\mathcal{T}|^2 \int_{-\infty}^{\infty} d\epsilon \, D_{N0}(\epsilon) D_{N2}(\epsilon + eV_z)[1 - \Theta(\epsilon)]\Theta(\epsilon + eV_z) = G_N V_z, \tag{S71}$$

where $G_N = e^2|\mathcal{T}|^2 D_{N0}(0) D_{N2}(0)/h$ is the conductance for normal metal state.

As indicated by Ref. [1], besides the CDW state of the 0+ Landau band, there is another Ohmic channel on the Fermi surface, likely due to the broadened band bottom of the +1 band which last till $B = 1.7$ T. Therefore, the tunneling current and differential resistance in this region at extremely low temperatures can be set in parallel as [5, 17, 24]

$$I_z = I_{cdw} + I_N, \tag{S72}$$

$$R_z = \frac{dV_z}{dI_z} = \frac{1}{G_{cdw} + G_N}. \tag{S73}$$

In order to compare with the experiment data [1], we plot the differential resistance as a function of tunneling current along the $z$-direction at the magnetic field $B = 1.55$ T for different temperatures as shown in Fig. 4 (f,g) in the main text. $T = 1.5$ K corresponds to the solid red line and $T = 2.5$ K corresponds to the solid orange line. The numerical results show a non-Ohmic $I_z - V_z$ character due to the CDW depinning. It is found that the threshold of the tunneling current is about 450 $\mu$A, which is consistent with the experiment [1] (please see the supplementary Figure 22 (b) of Ref. [1]). Particularly, we can obtain the value of the electron-phonon coupling constant $g_0 = 537.3$ eV·nm$^{-1}$ by comparing with the experimental data.

Notice that we use the following phenomenological tunneling model to fit the experiment. At $T = 1.5$ K, we have

$$I_z = \begin{cases} I_{cdw}^{(1)}(T) + I_N^{(1)}, & I_z < I_{th}; \\ I_{cdw}^{(2)}(\alpha_1 T) + I_N^{(2)}, & I_z > I_{th}, \end{cases} \tag{S74}$$

where $I_{th}$ is the threshold current, $\alpha_1 T$ is caused by the joule heat in the experiment with the fitting parameters $\alpha_1 = 7$, $G_{cdw}^{(1)} = 322.58$ m$\Omega^{-1}$, $G_N^{(1)} = 16.64$ m$\Omega^{-1}$, $G_{cdw}^{(2)} = 293.25$ m$\Omega^{-1}$, and $G_N^{(2)} = 49.75$ m$\Omega^{-1}$.

At $T = 2.5$ K, we have $I_z = I_{cdw}^{(3)}(\alpha_2 T) + I_N^{(3)}$, where $\alpha_2 T$ is caused by the Joule heat in the experiment with the fitting parameters $\alpha_2 = 5$, $G_{cdw}^{(3)} = 294.12$ m$\Omega^{-1}$, and $G_N^{(3)} = 53.76$ m$\Omega^{-1}$.


[1] F. Tang, Y. Ren, P. Wang, R. Zhong, J. Schneeloch, S. A. Yang, *et al.*, "Three-dimensional quantum Hall effect and metal-insulator transition in $ZrTe_5$", Nature **569**, 537 (2019).

[2] R. Y. Chen, Z. G. Chen, X.-Y. Song, J. A. Schneeloch, G. D. Gu, F. Wang, and N. L. Wang, "Magnetoinfrared spectroscopy of Landau levels and Zeeman splitting of three-dimensional massless Dirac fermions in $ZrTe_5$", Phys. Rev. Lett. **115**, 176404 (2015).

[3] Y. Jiang, Z. L. Dun, H. D. Zhou, Z. Lu, K.-W. Chen, S. Moon, *et al.*, "Landau-level spectroscopy of massive Dirac fermions in single-crystalline $ZrTe_5$ thin flakes", Phys. Rev. B **96**, 041101(R) (2017).

[4] J. L. Zhang, C. M. Wang, C. Y. Guo, X. D. Zhu, Y. Zhang, J. Y. Yang, *et al.*, "Anomalous thermoelectric effects of $ZrTe_5$ in and beyond the quantum limit", Phys. Rev. Lett. **123**, 196602 (2019).

[5] G. Grüner, *Density Waves in Solids* (Perseus, 2000).

[6] T. Giamarch, *Quantum Physics in one dimension* (Oxford, 2004).

[7] P. Coleman, *Introduction to Many-Body Physics* (Cambridge University Press, 2015).

[8] P. A. Lee, T. M. Rice, and P. W. Anderson, "Fluctuation effects at a Peierls transition", Phys. Rev. Lett. **31**, 462 (1973).

[9] A. P. Levanyuk, "Contribution to the theory of light scattering near the second-order phase transition points", J. Exp. Theor. Phys. **36**, 571 (1959).

[10] V. L. Ginzburg, "Some remarks on phase transitions of the second kind and the microscopic theory of ferroelectrics", J. Exp. Theor. Phys. **2**, 1824 (1960).

[11] H. Bruus and K. Flensberg, *Many-Body Quantum Theory in Condensed Matter Physics: An Introduction* (Oxford Graduate Texts, 2004).
[12] Z. Song, Z. Fang, and X. Dai, "Instability of Dirac semimetal phase under a strong magnetic field", Phys. Rev. B **96**, 235104 (2017).
[13] Z. Pan and R. Shindou, "Ground-state atlas of a three-dimensional semimetal in the quantum limit", Phys. Rev. B **100**, 165124 (2019).
[14] R. A. Jishi, *Feynman Diagram Techniques in Condensed Matter Physics* (Cambridge University Press, 2013).
[15] A. A. Abrikosov, "Quantum magnetoresistance", Phys. Rev. B **58**, 2788 (1998).
[16] B. Roy, J. D. Sau, and S. Das Sarma, "Migdal's theorem and electron-phonon vertex corrections in Dirac materials", Phys. Rev. B **89**, 165119 (2014).
[17] G. Grüner, "The dynamics of charge-density waves", Rev. Mod. Phys. **60**, 1129 (1988).
[18] R. K. Pathria, *Statistical Mechanics*, 2nd ed. (Butterworth-Heinemann Oxford, 1996).
[19] S. Kagoshima, H. Nagasawa, and T. Sambongi, *One-Dimensional Conductors* (Springer, Berlin, Heidelberg, 1988).
[20] P. A. Lee, T. M. Rice, and P. W. Anderson, "Conductivity from charge or spin density waves", Solid State Communications **14**, 703 (1974).
[21] J. Bardeen, "Theory of non-Ohmic conduction from charge-density waves in $NbSe_3$", Phys. Rev. Lett. **42**, 1498 (1979).
[22] J. Bardeen, "Tunneling theory of charge-density-wave depinning", Phys. Rev. Lett. **45**, 1978 (1980).
[23] G. D. Mahan, *Many-Particle Physics*, 3rd ed., Physics of Solids and Liquids (Springer Science & Business Media New York, 2000).
[24] G. Grüner and A. Zettl, "Charge density wave conduction: A novel collective transport phenomenon in solids", Physics Reports **119**, 117 (1985).
